# Supplementary material for: Deep Relevance Ranking Using Enhanced Document-Query Interactions
Source: arXiv:1809.01682 ancillary file (2018-09-11)
Supplement: Supplementary file 1 [file supplementary_material.pdf]

# Deep Relevance Ranking Using Enhanced Document-Query Interactions Supplementary Material

**Ryan McDonald**[1,2], **Georgios-Ioannis Brokos**[1] and **Ion Androutsopoulos**[1]

[1]Dept. of Informatics, Athens University of Economics and Business, Greece
[2]Google AI

## Appendix A: Hyperparameters

### Word2Vec

For both datasets, we used the GenSim[1] implementation of word2vec (skip-gram model), with negative sampling, window size set to 5, default other hyper-parameter values, to produce word embeddings of $r = 200$ and $r = 30$ dimensions. The word embeddings were not updated when training the document relevance ranking models.

### PACRR Models

Both PACRR and PACRR-DRMM used a learning rate of 0.001 and $\beta_1/\beta_2 = 0.9/0.999$ with batch size equal to 32. Following Hui et al. (2018), we used binary log-loss over pairs of a single positive and a single negative document of the same query.

Maximum query length $l_q$ was set to 30 for BIOASQ and 5 for TREC ROBUST. Maximum document length $l_d$ was set to 300 and 1000 for each dataset, respectively, values that are larger than 92% and 90% of the documents of each dataset, respectively. Maximum kernel size $(l_g \times l_g)$ was set to $(3 \times 3)$ with number of filters per size $n_f = 16$. Row-wise $k$-max pooling used $k = 2$.

PACRR used a 2-layer MLP with RELU activations and hidden layers with 70 dimensions to score the document-aware query representation, while PACRR-DRMM used a 2-layer MLP with RELU activations and hidden layers with 7 dimensions to independently score each document-aware query-term encoding. The input embeddings used $r = 200$ dimension.

### DRMM Models

All DRMM models used a learning rate of 0.01 and $\beta_1/\beta_2 = 0.9/0.999$. Gradient clipping with a threshold of 5.0 was used. Batch sizes were set to 32, as in the original DRMM papers. We used a hinge-loss with a margin of 1.0 over pairs of a single positive and a single negative document of the same query. All DRMM models, unless otherwise specified, used a 2-layer q-term scoring MLP with leaky-RELU activation functions and 8 dimension per hidden layer.

The input embeddings used $r = 30$ dimension as we found these were faster and even sometimes more accurate. For context-sensitive term encodings we used an LSTM with 2 layers and hidden dimension of 30. We used a dropout of 0.3 on the input and hidden layers of the LSTMs.

For the DRMM baseline, we used 30 histogram buckets, following Guo et al. (2016). We experimented with different count encodings and used log-counts in each bucket, as in the original paper.

In the basic POSIT-DRMM (not the multi-view variant), since the document-aware q-term encoding is 2-dimensional, we used a single layer (instead of 2 layers) for q-term relevance scoring. For the $k$-max pooling operation, we set $k = 5$.

### All Relevance Ranking Models

Parameters are initialized using the method of Glorot and Bengio (2010), thought we found little difference in initialization strategies. No dropout was applied anywhere besides the LSTM layers as it did not help empirically.

## Appendix B: Evaluation resources

### Dataset statistics

Table 1 summarizes the statistics for both the BIOASQ and TREC ROBUST 2004 datasets.

Table 2 reports further statistics about the relevant documents per query in the two datasets.

[1]Consult https://radimrehurek.com/gensim/models/word2vec.html. We used v. 3.3.0.

| | BIOASQ | ROBUST |
|---|---|---|
| Number of queries | 2,251 | 250 |
| Avg. query length (Tokens) | 9.16 | 2.74 |
| Collection size (Documents) | 17.7M | 528K |
| Collection size (Tokens) | 3.5B | 252M |
| Avg. doc. length (Tokens) | 196.6 | 476.5 |
| Vocabulary | 15.2M | 1.4M |
| Word2vec vocabulary | 2.7M | 322K |

Table 1: Dataset statistics.

| **Relevant Docs** | BIOASQ | ROBUST |
|---|---|---|
| Average | 12.0 | 69.6 |
| Min | 1 | 0 |
| Max | 157 | 448 |
| St.Dev. | 11.1 | 74.4 |

Table 2: Relevant documents per query.

## Significance testing

For stratified shuffling we used $10,000$ runs and $p < 0.05$ as the threshold. We sometimes stopped the number of runs at $1,000$ if $p < 0.01$ or $p > 0.1$ since we never observed these values crossing the $0.05$ threshold after that point.

## References


Xavier Glorot and Yoshua Bengio. 2010. Understanding the difficulty of training deep feedforward neural networks. In *Proceedings of the Thirteenth International Conference on Artificial Intelligence and Statistics*, pages 249–256, Sardinia, Italy.

Jiafeng Guo, Yixing Fan, Qingyao Ai, and W Bruce Croft. 2016. A deep relevance matching model for ad-hoc retrieval. In *Proceedings of the 25th ACM International on Conference on Information and Knowledge Management*, pages 55–64, Indianapolis, IN.

Kai Hui, Andrew Yates, Klaus Berberich, and Gerard de Melo. 2018. Co-PACRR: A context-aware neural IR model for ad-hoc retrieval. In *Proceedings of the 11th ACM International Conference on Web Search and Data Mining*, pages 279–287, Marina Del Rey, CA.
